# Supplementary material for: A Review of Neuroscience-Inspired Machine Learning
Source: arXiv:2403.18929 source file (2024-02-16)
Supplement: Supplementary file 1 [file appendix.tex]

\subsection*{Feedback Alignment} % and Sign Symmetry} 
\label{sec:feedback_alignment}

\paragraph{Background.} The general premise behind schemes that fall could be considered as conducting a form of feedback alignment is that the adjustment of parameter values in an ANN did not require the use of symmetric forward and backward connections or feedback pathways. In effect, feedback alignment approaches address the problem of weight-transport in backprop-based ANNs. Notably, in \cite{lillicrap2016random}, one of the earliest forms of this type of credit assignment, i.e., random feedback alignment, demonstrated that it was possible to utilize fixed, random feedback projections to generate the teaching signals for each layer. Further variations to this theme led to the construction of training algorithms by introducing random matrices that directly propagated random projections of the output error to individual layers directly \cite{nokland2016direct}, e.g., direct and indirect feedback alignment. %This is interesting, as feedback alignment allows to perform machine learning tasks via forward passes only, a fundamental property for implementations on photonic chips \cite{launay2020hardware,filipovich2022silicon}. 

Desirably, direct feedback alignment (DFA) has further been shown to scale to large-scale datasets  \cite{moskovitz2018feedback,launay2020direct} (in the context of classification) and a key generalization of feedback alignment \cite{liao2016important}, i.e., sign symmetry, facilitate the adaptation of the feedback pathways themselves, forcing these connections to share the same signs but not the same magnitudes as the forward ones. Note that, despite its lack of theoretical justification (they do not result in accurate transmission/propagation of the error gradients), sign symmetry-based approaches have been empirically demonstrated to offer only slightly worse performance than backprop, including in architectures that utilize convolutional tensor connections  \cite{xiao2018biologically}.

\paragraph{Energy Functional.} The functional that a feedback alignment process typically optimizes could be written down as:
\begin{align}
    \mathcal{F}(\Theta) = \beta \mathcal{L}(\Theta)\Big|_{\beta=1} + \alpha \mathcal{E}(\Theta)\Big|_{\alpha=0} = \mathcal{L}(\Theta)
\end{align}
where we notice that the weight on the outer (supervised) component of the objective is set to one and the internal (unsupervised) component is evaluated at zero.

\paragraph{Mechanics.} \textcolor{red}{WRITEME:}

\subsection*{Target Propagation and Alignment of Distributed Representations} % cite/mention recircation as early predecessor

\paragraph{Background.}
A primary distinguishing feature of the framework of target propagation (targetprop) is that, instead of gradients, target (vector) signals are backpropagated throughout a neural system. In effect, each pair of layers in a neural network are treated as a shallow autoencoder; each layer tries to reconstruct the one below it, specifically seeking to learn a local function and its (approximate) inversion. Each autoencoder is designed with separate forward and backward synaptic connections and local rules are used to adjust the values within each. Usefully, targetprop has seen application to the learning of temporal and sequential structure, e.g., tasks in natural language processing \cite{manchev2020target,wiseman2017training,mali2021investigating}. %In all cases, however, the performance is not comparable to backprop's. 

Theoretically, it has been shown that targetprop is related to a form of Gaussian-Newton optimization \cite{meulemans20}, where variations of targetprop that hybridize/combine aspects of gradient descent and Gauss-Netwon adjustments have been proposed to improve overall performance; this comes at the cost of some biological plausibility. Efforts such as \cite{ernoult2022} further modify targetprop to learn/produce target signals that are similar to the gradients yielded by backprop, further improving performance and restoring biological plausibility; the local objective is modified by introducing a term that pushes the Jacobian of the inversion/decoder parameters to move closer to that of the feedforward/encoder parameters. In other instances, it has been shown the inversion parameters can be kept random and fixed (similar in style to feedback alignment pathways) \cite{shibuya2022fixed}. %Thus targetprop can be considered as an approximation of predictive coding, where instead of local loss, targets are pushed. Thus, assuming the underlying function to be approximated is Lipschitz continuous, and the difference between forward and backward activity is less than some $\epsilon$ (where $\epsilon$ is some small value), the network can be shown to converge to an optimal point. In predictive coding, this is achieved by minimizing an energy function over an arbitrary number inference steps, which empirically reduces uncertainty and leads to a stable and robust performance.

%% LRA
The framework of local representation alignment \cite{ororbia2019biologically} (LRA) can be viewed as a hybrid between targetprop and predictive coding (reviewed later), building on a form of `coordinated local learning' that, in essence, results in the minimization of an objective that is the sum of local representation distance measurements \cite{ororbia2019biologically}. LRA-based approaches, in the context of classification in computer vision tasks, have been shown to generalize well on large-scale (image) benchmarks such as CIFAR-10 and ImageNet \cite{ororbia2020large,zee2022robust}. Like targetprop, under mild assumptions, it can be shown that LRA approximates backprop \cite{ororbia2018conducting}.

\paragraph{Energy Functional.} The functional that targetprop could be viewed as optimizing is:
\begin{alignat}{3}
    \mathcal{F}(\Theta) &= \beta \mathcal{L}(\Theta)\Big|_{\beta=1} &&+ \alpha \mathcal{E}(\Theta)\Big|_{\alpha=1} \\
    &= \mathcal{L}(\Theta_L) + \sum^{L-1}_{\ell=1}&& \Big( ||f_{\Theta_\ell}(\mathbf{z}^{\ell-1}) - \mathbf{\hat{z}}^\ell ||^p_q \nonumber \\
    & &&+ ||\mathbf{z}^\ell - d_{\Theta_\ell}(f_{\Theta_\ell}(\mathbf{z}^\ell))||^p_q \Big)
\end{alignat}
where we see within the energy functional the emphasis placed on the internal structure of the neural system to be made up of coupled encoding $f()$ and decoding $d()$ functions. Further notice that the outer term of targetprop focuses the outer supervised objective on the topmost parameters $\Theta_L$.

Local representation alignment schemes, which share similarities to targetprop (but are regarded more as a hybridization of principles underlying targetprop and predictive coding \cite{rao1999predictive}), follow a different and simpler internal energy functional:
\begin{align}
    \mathcal{E}(\Theta) = \sum^{L-1}_{\ell=1} ||f_{\Theta_\ell}(\mathbf{z}^{\ell-1}) - \phi^\ell(\mathbf{h}^\ell - \gamma d_{\Theta_\ell}(\mathbf{e}^{\ell+1}))||^p_q
\end{align}
where we observe that the decoding function actually projects the local mismatch of the encoding/decoding pairing above.

\paragraph{Mechanics.} \textcolor{red}{WRITEME:}
